# Supplementary material for: Open-shell Tensor Hypercontraction
Source: arXiv:2304.04040 ancillary file (2023-05-27)
Supplement: Supplementary file 1 [file si.pdf]

# Open-shell Tensor Hypercontraction: Electronic Supplementary Information

Tingting Zhao,[†,‡] Megan Simons,[†,‡] and Devin A. Matthews[*,‡]

†*These authors contributed equally to this work.*

‡*Department of Chemistry, Southern Methodist University, Dallas, TX*

E-mail: damatthews@smu.edu

## Factorized LS-THC-MP3 equations

The notation used here is the same as in the main text, except that we disambiguate the core matrix $\mathbf{V}$ based on which collocation matrices are applied; for example $\mathbf{V}^{(pqrs)}$ is the specific core matrix indicated by $X_p^R X_r^R V_{RS} X_q^S X_s^S$. Including the various spin cases, this leads to a total of 13 distinct core matrices,

$$V_{RS}^{(ijkl)} \rightarrow V_{RS}, \quad V_{R\bar{S}}^{(ij\bar{k}\bar{l})} \rightarrow V_{R\bar{S}}, \quad V_{\bar{R}\bar{S}}^{(\bar{i}\bar{j}\bar{k}\bar{l})} \rightarrow V_{\bar{R}\bar{S}} \tag{1}$$

$$V_{RS}^{(abij)} \rightarrow \tilde{V}_{RS}, \quad V_{R\bar{S}}^{(a\bar{b}i\bar{j})} \rightarrow \tilde{V}_{R\bar{S}}, \quad V_{\bar{R}\bar{S}}^{(\bar{a}\bar{b}\bar{i}\bar{j})} \rightarrow \tilde{V}_{\bar{R}\bar{S}} \tag{2}$$

$$V_{RS}^{(abcd)} \rightarrow \tilde{\tilde{V}}_{RS}, \quad V_{R\bar{S}}^{(a\bar{b}c\bar{d})} \rightarrow \tilde{\tilde{V}}_{R\bar{S}}, \quad V_{\bar{R}\bar{S}}^{(\bar{a}\bar{b}\bar{c}\bar{d})} \rightarrow \tilde{\tilde{V}}_{\bar{R}\bar{S}} \tag{3}$$

$$V_{RS}^{(aibj)} \rightarrow \bar{V}_{RS}, \quad V_{R\bar{S}}^{(a\bar{i}b\bar{j})} \rightarrow \bar{V}_{R\bar{S}}, \quad V_{\bar{R}S}^{(\bar{a}i\bar{b}j)} \rightarrow \bar{V}_{\bar{R}S}, \quad V_{\bar{R}\bar{S}}^{(\bar{a}\bar{i}\bar{b}\bar{j})} \rightarrow \bar{V}_{\bar{R}\bar{S}} \tag{4}$$

Note that for the $ijkl$, $abij$, and $abcd$ distributions the mixed spin cases are symmetrically defined, e.g. $\tilde{V}_{\bar{R}S} = \tilde{V}_{S\bar{R}}$.

The factorized equations for the LS-THC-MP3b energy correction utilize the following

intermediates,

$$P_{ij}^{R} = \sum_{S} V_{RS} X_i^S X_j^S, \quad P_{ij}^{\bar{R}} = \sum_{S} V_{\bar{R}S} X_i^S X_j^S, \tag{5}$$

$$P_{\bar{i}\bar{j}}^{R} = \sum_{\bar{S}} V_{R\bar{S}} X_i^{\bar{S}} X_j^{\bar{S}}, \quad P_{\bar{i}\bar{j}}^{\bar{R}} = \sum_{\bar{S}} V_{\bar{R}\bar{S}} X_i^{\bar{S}} X_j^{\bar{S}} \tag{6}$$

$$\tilde{P}_{ai}^{R} = \sum_{S} \tilde{V}_{RS} \tilde{X}_a^S \tilde{X}_i^S, \quad \tilde{P}_{ai}^{\bar{R}} = \sum_{S} \tilde{V}_{\bar{R}S} \tilde{X}_a^S \tilde{X}_i^S, \tag{7}$$

$$\tilde{P}_{\bar{a}\bar{i}}^{R} = \sum_{\bar{S}} \tilde{V}_{R\bar{S}} \tilde{X}_a^{\bar{S}} \tilde{X}_i^{\bar{S}}, \quad \tilde{P}_{\bar{a}\bar{i}}^{\bar{R}} = \sum_{\bar{S}} \tilde{V}_{\bar{R}\bar{S}} \tilde{X}_a^{\bar{S}} \tilde{X}_i^{\bar{S}} \tag{8}$$

$$\bar{P}_{ij}^{R} = \sum_{S} \bar{V}_{RS} X_i^S X_j^S, \quad \bar{P}_{ij}^{\bar{R}} = \sum_{S} \bar{V}_{\bar{R}S} X_i^S X_j^S, \tag{9}$$

$$\bar{P}_{\bar{i}\bar{j}}^{R} = \sum_{\bar{S}} \bar{V}_{R\bar{S}} X_i^{\bar{S}} X_j^{\bar{S}}, \quad \bar{P}_{\bar{i}\bar{j}}^{\bar{R}} = \sum_{\bar{S}} \bar{V}_{\bar{R}\bar{S}} X_i^{\bar{S}} X_j^{\bar{S}} \tag{10}$$

$$\tilde{\tilde{P}}_{ai}^{R} = \sum_{S} \tilde{\tilde{V}}_{RS} \tilde{\tilde{X}}_a^S \tilde{\tilde{X}}_i^S, \quad \tilde{\tilde{P}}_{ai}^{\bar{R}} = \sum_{S} \tilde{\tilde{V}}_{\bar{R}S} \tilde{\tilde{X}}_a^S \tilde{\tilde{X}}_i^S, \tag{11}$$

$$\tilde{\tilde{P}}_{\bar{a}\bar{i}}^{R} = \sum_{\bar{S}} \tilde{\tilde{V}}_{R\bar{S}} \tilde{\tilde{X}}_a^{\bar{S}} \tilde{\tilde{X}}_i^{\bar{S}}, \quad \tilde{\tilde{P}}_{\bar{a}\bar{i}}^{\bar{R}} = \sum_{\bar{S}} \tilde{\tilde{V}}_{\bar{R}\bar{S}} \tilde{\tilde{X}}_a^{\bar{S}} \tilde{\tilde{X}}_i^{\bar{S}} \tag{12}$$

$$Q_{ai}^{R} = \sum_{S} T_{RS}^{[1]} \tilde{X}_a^S \tilde{X}_i^S, \quad Q_{ai}^{\bar{R}} = \sum_{S} T_{\bar{R}S}^{[1]} \tilde{X}_a^S \tilde{X}_i^S, \tag{13}$$

$$Q_{\bar{a}\bar{i}}^{R} = \sum_{\bar{S}} T_{R\bar{S}}^{[1]} \tilde{X}_a^{\bar{S}} \tilde{X}_i^{\bar{S}}, \quad Q_{\bar{a}\bar{i}}^{\bar{R}} = \sum_{\bar{S}} T_{\bar{R}\bar{S}}^{[1]} \tilde{X}_a^{\bar{S}} \tilde{X}_i^{\bar{S}} \tag{14}$$

$$WXX^{QU} = \sum_{P} T_{QP}^{[1]} ((\sum_{a} X_a^P X_a^U)(\sum_{i} X_i^P X_i^U)) \tag{15}$$

$$WXX^{Q\bar{U}} = \sum_{\bar{P}} T_{Q\bar{P}}^{[1]} ((\sum_{a} X_a^{\bar{P}} X_a^{\bar{U}})(\sum_{i} X_i^{\bar{P}} X_i^{\bar{U}})) \tag{16}$$

$$WXX^{\bar{Q}U} = \sum_{P} T_{\bar{Q}P}^{[1]} ((\sum_{a} X_a^P X_a^U)(\sum_{i} X_i^P X_i^U)) \tag{17}$$

$$WXX^{\bar{Q}\bar{U}} = \sum_{\bar{P}} T_{\bar{Q}\bar{P}}^{[1]} ((\sum_{a} X_a^{\bar{P}} X_a^{\bar{U}})(\sum_{i} X_i^{\bar{P}} X_i^{\bar{U}})) \tag{18}$$

$$VXX^{SQ} = \sum_{R} V_{RS} (\sum_{e} X_e^R X_e^Q)(\sum_{m} X_m^R X_m^Q) \tag{19}$$

$$VXX^{S\bar{Q}} = \sum_{\bar{R}} V_{\bar{R}S} (\sum_{e} X_e^{\bar{R}} X_e^{\bar{Q}})(\sum_{m} X_m^{\bar{R}} X_m^{\bar{Q}}) \tag{20}$$

$$VXX^{\bar{S}Q} = \sum_{R} V_{R\bar{S}}(\sum_{e} X_e^R X_e^Q)(\sum_{m} X_m^R X_m^Q) \tag{21}$$

$$VXX^{\bar{S}\bar{Q}} = \sum_{\bar{R}} V_{\bar{R}\bar{S}}(\sum_{e} X_e^{\bar{R}} X_e^{\bar{Q}})(\sum_{m} X_m^{\bar{R}} X_m^{\bar{Q}}) \tag{22}$$

The LS-THC-MP3b energy itself is term-by-term,

$$E_{PPC} = \frac{1}{2}\sum_{Ubj}(\sum_{S}(\sum_{Q}(\sum_{e}(\sum_{a} \tilde{\tilde{P}}_{ae}^{S} \tilde{X}_a^U)(\sum_{i} Q_{ei}^P \tilde{X}_i^U))(\sum_{f} \tilde{\tilde{X}}_f^S \tilde{X}_f^Q)\tilde{X}_j^Q)\tilde{\tilde{X}}_b^S)Q_{bj}^U \tag{23}$$

$$+\frac{1}{2}\sum_{Ubj}(\sum_{\bar{S}}(\sum_{\bar{Q}}(\sum_{e}(\sum_{a} \tilde{\tilde{P}}_{ae}^{\bar{S}} \tilde{X}_a^U)(\sum_{i} Q_{ei}^P \tilde{X}_i^U))(\sum_{f} \tilde{\tilde{X}}_f^{\bar{S}} \tilde{X}_f^{\bar{Q}})\tilde{X}_j^{\bar{Q}})\tilde{\tilde{X}}_b^{\bar{S}})Q_{bj}^U \tag{24}$$

$$+\frac{1}{2}\sum_{\bar{U}}\bar{b}\bar{j}(\sum_{S}(\sum_{Q}(\sum_{\bar{e}}(\sum_{\bar{a}} \tilde{\tilde{P}}_{\bar{a}\bar{e}}^{S} \tilde{X}_a^{\bar{U}})(\sum_{i} Q_{\bar{e}\bar{i}}^P \tilde{X}_i^{\bar{U}}))(\sum_{f} \tilde{\tilde{X}}_f^S \tilde{X}_f^Q)\tilde{X}_j^Q)\tilde{\tilde{X}}_b^S)Q_{bj}^{\bar{U}} \tag{25}$$

$$+\frac{1}{2}\sum_{\bar{U}}\bar{b}\bar{j}(\sum_{\bar{S}}(\sum_{\bar{Q}}(\sum_{e}(\sum_{a} \tilde{\tilde{P}}_{\bar{a}\bar{e}}^{\bar{S}} \tilde{X}_a^{\bar{U}})(\sum_{i} Q_{\bar{e}\bar{i}}^{\bar{P}} \tilde{X}_i^{\bar{U}}))(\sum_{f} \tilde{\tilde{X}}_f^{\bar{S}} \tilde{X}_f^{\bar{Q}})\tilde{X}_j^{\bar{Q}})\tilde{\tilde{X}}_b^{\bar{S}})Q_{bj}^{\bar{U}} \tag{26}$$

$$E_{PPX} = -\frac{1}{2}\sum_{QRV}(\sum_{f}(\sum_{b} \tilde{\tilde{P}}_{bf}^{R} \tilde{X}_b^V)\tilde{X}_f^Q)\sum_{i}(\sum_{e} Q_{ei}^Q \tilde{\tilde{X}}_e^R)\tilde{X}_i^V)\sum_{j}(\sum_{a} Q_{aj}^V \tilde{\tilde{X}}_a^R)\tilde{X}_j^Q) \tag{27}$$

$$-\frac{1}{2}\sum_{\bar{Q}\bar{R}\bar{V}}(\sum_{f}(\sum_{b} \tilde{\tilde{P}}_{bf}^{\bar{R}} \tilde{X}_b^{\bar{V}})\tilde{X}_f^{\bar{Q}})\sum_{i}(\sum_{e} Q_{ei}^{\bar{Q}} \tilde{\tilde{X}}_e^{\bar{R}})\tilde{X}_i^{\bar{V}})\sum_{j}(\sum_{a} Q_{aj}^{\bar{V}} \tilde{\tilde{X}}_a^{\bar{R}})\tilde{X}_j^{\bar{Q}}) \tag{28}$$

$$E_{HHC} = \frac{1}{2}\sum_{Ubj}(\sum_{S}(\sum_{Q}(\sum_{m}(\sum_{i} P_{im}^S \tilde{X}_i^U)(\sum_{a} Q_{am}^P \tilde{X}_a^U))(\sum_{n} X_n^S \tilde{X}_n^Q)X_j^S)\tilde{X}_b^Q)Q_{bj}^U \tag{29}$$

$$+\frac{1}{2}\sum_{Ubj}(\sum_{\bar{S}}(\sum_{\bar{Q}}(\sum_{m}(\sum_{i} P_{im}^{\bar{S}} \tilde{X}_i^U)(\sum_{a} Q_{am}^P \tilde{X}_a^U))(\sum_{n} X_n^{\bar{S}} \tilde{X}_n^{\bar{Q}})X_j^{\bar{S}})\tilde{X}_b^{\bar{Q}})Q_{bj}^U \tag{30}$$

$$+\frac{1}{2}\sum_{\bar{U}}\bar{b}\bar{j}(\sum_{S}(\sum_{Q}(\sum_{\bar{m}}(\sum_{\bar{i}} P_{\bar{i}\bar{m}}^S \tilde{X}_i^{\bar{U}})(\sum_{a} Q_{\bar{a}\bar{m}}^P \tilde{X}_a^{\bar{U}}))(\sum_{n} X_n^S \tilde{X}_n^Q)X_j^S)\tilde{X}_b^Q)Q_{bj}^{\bar{U}} \tag{31}$$

$$+\frac{1}{2}\sum_{\bar{U}}\bar{b}\bar{j}(\sum_{\bar{S}}(\sum_{\bar{Q}}(\sum_{m}(\sum_{i} P_{\bar{i}\bar{m}}^{\bar{S}} \tilde{X}_i^{\bar{U}})(\sum_{a} Q_{\bar{a}\bar{m}}^{\bar{P}} \tilde{X}_a^{\bar{U}}))(\sum_{n} X_n^{\bar{S}} \tilde{X}_n^{\bar{Q}})X_j^{\bar{S}})\tilde{X}_b^{\bar{Q}})Q_{bj}^{\bar{U}} \tag{32}$$

$$E_{HHX} = -\frac{1}{2}\sum_{QRV}(\sum_{n}(\sum_{j} P_{jn}^R \tilde{X}_j^V)\tilde{X}_n^Q)\sum_{m}(\sum_{a} Q_{am}^Q \tilde{X}_a^V)X_m^R)\sum_{i}(\sum_{b} Q_{bi}^V \tilde{X}_b^Q)X_i^R) \tag{33}$$

$$-\frac{1}{2}\sum_{\bar{Q}\bar{R}\bar{V}}(\sum_{n}(\sum_{j} P_{jn}^{\bar{R}} \tilde{X}_j^{\bar{V}})\tilde{X}_n^{\bar{Q}})\sum_{m}(\sum_{a} Q_{am}^{\bar{Q}} \tilde{X}_a^{\bar{V}})X_m^{\bar{R}})\sum_{i}(\sum_{b} Q_{bi}^{\bar{V}} \tilde{X}_b^{\bar{Q}})X_i^{\bar{R}}) \tag{34}$$

$$E_{PH1} = WXX^{QU}WXX^{US}VXX^{SQ} \tag{35}$$

$$+WXX^{Q\bar{U}}WXX^{\bar{U}S}VXX^{SQ} \tag{36}$$

$$+WXX^{QU}WXX^{U\bar{S}}VXX^{\bar{S}Q} \tag{37}$$

$$+WXX^{\bar{Q}U}WXX^{US}VXX^{S\bar{Q}} \tag{38}$$

$$+WXX^{\bar{Q}U}WXX^{U\bar{S}}VXX^{\bar{S}\bar{Q}} \tag{39}$$

$$+WXX^{\bar{Q}\bar{U}}WXX^{\bar{U}S}VXX^{S\bar{Q}} \tag{40}$$

$$+WXX^{Q\bar{U}}WXX^{\bar{U}\bar{S}}VXX^{\bar{S}Q} \tag{41}$$

$$+WXX^{\bar{Q}\bar{U}}WXX^{\bar{U}\bar{S}}VXX^{\bar{S}\bar{Q}} \tag{42}$$

$$E_{PH2} = -\sum_{PV}(\sum_{bj}(\sum_{Q}(\sum_{R}(\sum_{m}\bar{P}^{R}_{mj}\tilde{X}^{Q}_{m})(\sum_{e}\tilde{\tilde{X}}^{R}_{e}\tilde{X}^{Q}_{e})\tilde{\tilde{X}}^{R}_{b})T^{[1]}_{QP})\tilde{X}^{V}_{b}\tilde{X}^{V}_{j})(ST^{[1]})_{VP} \tag{43}$$

$$-\sum_{\bar{P}V}(\sum_{bj}(\sum_{Q}(\sum_{R}(\sum_{m}\bar{P}^{\bar{R}}_{mj}\tilde{X}^{Q}_{m})(\sum_{e}\tilde{\tilde{X}}^{R}_{e}\tilde{X}^{Q}_{e})\tilde{\tilde{X}}^{R}_{b})T^{[1]}_{Q\bar{P}})\tilde{X}^{V}_{b}\tilde{X}^{V}_{j})(ST^{[1]})_{V\bar{P}} \tag{44}$$

$$-\sum_{P\bar{V}}(\sum_{\bar{b}\bar{j}}(\sum_{\bar{Q}}(\sum_{\bar{R}}(\sum_{\bar{m}}\bar{P}^{\bar{R}}_{\bar{m}\bar{j}}\tilde{X}^{\bar{Q}}_{\bar{m}})(\sum_{\bar{e}}\tilde{\tilde{X}}^{\bar{R}}_{\bar{e}}\tilde{X}^{\bar{Q}}_{\bar{e}})\tilde{\tilde{X}}^{\bar{R}}_{\bar{b}})T^{[1]}_{\bar{Q}P})\tilde{X}^{\bar{V}}_{\bar{b}}\tilde{X}^{\bar{V}}_{\bar{j}})(ST^{[1]})_{\bar{V}P} \tag{45}$$

$$-\sum_{\bar{P}\bar{V}}(\sum_{\bar{b}\bar{j}}(\sum_{\bar{Q}}(\sum_{\bar{R}}(\sum_{\bar{m}}\bar{P}^{\bar{R}}_{\bar{m}\bar{j}}\tilde{X}^{\bar{Q}}_{\bar{m}})(\sum_{\bar{e}}\tilde{\tilde{X}}^{\bar{R}}_{\bar{e}}\tilde{X}^{\bar{Q}}_{\bar{e}})\tilde{\tilde{X}}^{\bar{R}}_{\bar{b}})T^{[1]}_{\bar{Q}\bar{P}})\tilde{X}^{\bar{V}}_{\bar{b}}\tilde{X}^{\bar{V}}_{\bar{j}})(ST^{[1]})_{\bar{V}\bar{P}} \tag{46}$$

$$E_{PH3} = -\sum_{Ubj}(\sum_{R}(\sum_{Q}(\sum_{m}(\sum_{i}\bar{P}^{R}_{mi}\tilde{X}^{U}_{i})(\sum_{a}Q^{Q}_{am}\tilde{X}^{U}_{a}))(\sum_{e}\tilde{\tilde{X}}^{R}_{e}\tilde{X}^{Q}_{e})\tilde{X}^{Q}_{j})\tilde{\tilde{X}}^{R}_{b})Q^{U}_{bj} \tag{47}$$

$$-\sum_{\bar{U}}\bar{b}\bar{j}(\sum_{R}(\sum_{Q}(\sum_{\bar{m}}(\sum_{\bar{i}}\bar{P}^{R}_{\bar{m}\bar{i}}\tilde{X}^{\bar{U}}_{i})(\sum_{\bar{a}}Q^{Q}_{\bar{a}\bar{m}}\tilde{X}^{\bar{U}}_{a}))(\sum_{e}\tilde{\tilde{X}}^{R}_{e}\tilde{X}^{Q}_{e})\tilde{X}^{Q}_{j})\tilde{\tilde{X}}^{R}_{b})Q^{\bar{U}}_{bj} \tag{48}$$

$$-\sum_{U\bar{b}\bar{j}}(\sum_{\bar{R}}(\sum_{\bar{Q}}(\sum_{m}(\sum_{i}\bar{P}^{\bar{R}}_{mi}\tilde{X}^{U}_{i})(\sum_{a}Q^{\bar{Q}}_{am}\tilde{X}^{U}_{a}))(\sum_{\bar{e}}\tilde{\tilde{X}}^{\bar{R}}_{e}\tilde{X}^{\bar{Q}}_{e})\tilde{X}^{\bar{Q}}_{j})\tilde{\tilde{X}}^{\bar{R}}_{b})Q^{U}_{\bar{b}\bar{j}} \tag{49}$$

$$-\sum_{\bar{U}\bar{b}\bar{j}}(\sum_{\bar{R}}(\sum_{\bar{Q}}(\sum_{\bar{m}}(\sum_{\bar{i}}\bar{P}^{\bar{R}}_{\bar{m}\bar{i}}\tilde{X}^{\bar{U}}_{i})(\sum_{\bar{a}}Q^{\bar{Q}}_{\bar{a}\bar{m}}\tilde{X}^{\bar{U}}_{a}))(\sum_{\bar{e}}\tilde{\tilde{X}}^{\bar{R}}_{e}\tilde{X}^{\bar{Q}}_{e})\tilde{X}^{\bar{Q}}_{j})\tilde{\tilde{X}}^{\bar{R}}_{b})Q^{\bar{U}}_{\bar{b}\bar{j}} \tag{50}$$

$$E_{PH4} = \sum_{RS}(\sum_{ai}(\sum_{U}(\sum_{b}Q^{U}_{bi}\tilde{X}^{S}_{b})(\sum_{j}\tilde{X}^{U}_{j}\tilde{X}^{S}_{j})\tilde{X}^{U}_{a})(\sum_{P}(\sum_{e}Q^{P}_{ei}\tilde{X}^{R}_{e})(\sum_{m}\tilde{X}^{P}_{m}\tilde{X}^{R}_{m})\tilde{X}^{P}_{a}))\tilde{V}_{RS}$$

(51)

$$+\sum_{\bar{R}\bar{S}}(\sum_{\bar{a}\bar{i}}(\sum_{\bar{U}}(\sum_{\bar{b}}Q^{\bar{U}}_{\bar{b}\bar{i}}\tilde{X}^{\bar{S}}_{b})(\sum_{\bar{j}}\tilde{X}^{\bar{U}}_{j}\tilde{X}^{\bar{S}}_{j})\tilde{X}^{\bar{U}}_{a})(\sum_{\bar{P}}(\sum_{\bar{e}}Q^{\bar{P}}_{\bar{e}\bar{i}}\tilde{X}^{\bar{R}}_{e})(\sum_{\bar{m}}\tilde{X}^{\bar{P}}_{m}\tilde{X}^{\bar{R}}_{m})\tilde{X}^{\bar{P}}_{a}))\tilde{V}_{\bar{R}\bar{S}}$$

(52)

$$E_{PH5} = -\sum_{PR}(\sum_{ai}(\sum_{Q}(\sum_{U}(\sum_{b}Q^{U}_{bi}\tilde{X}^{S}_{b})(\sum_{j}\tilde{X}^{U}_{j}\tilde{X}^{S}_{j})\tilde{X}^{U}_{a})\tilde{V}_{RS})\tilde{X}^{P}_{a}\tilde{X}^{P}_{i})WXX^{PR} \tag{53}$$

$$- \sum_{P\bar{R}} (\sum_{ai} (\sum_{\bar{Q}} (\sum_{U} (\sum_{b} Q^{U}_{bi} \tilde{X}^{S}_{b}) (\sum_{j} \tilde{X}^{U}_{j} \tilde{X}^{S}_{j}) \tilde{X}^{U}_{a}) \tilde{V}_{\bar{R}S}) \tilde{X}^{P}_{a} \tilde{X}^{P}_{i}) WXX^{P\bar{R}} \quad (54)$$

$$- \sum_{\bar{P}R} (\sum_{\bar{a}\bar{i}} (\sum_{Q} (\sum_{\bar{U}} (\sum_{\bar{b}} Q^{\bar{U}}_{\bar{b}\bar{i}} \tilde{X}^{\bar{S}}_{b}) (\sum_{\bar{j}} \tilde{X}^{\bar{U}}_{j} \tilde{X}^{\bar{S}}_{j}) \tilde{X}^{\bar{U}}_{a}) \tilde{V}_{R\bar{S}}) \tilde{X}^{\bar{P}}_{a} \tilde{X}^{\bar{P}}_{i}) WXX^{\bar{P}R} \quad (55)$$

$$- \sum_{\bar{P}\bar{R}} (\sum_{\bar{a}\bar{i}} (\sum_{\bar{Q}} (\sum_{\bar{U}} (\sum_{\bar{b}} Q^{\bar{U}}_{\bar{b}\bar{i}} \tilde{X}^{\bar{S}}_{b}) (\sum_{\bar{j}} \tilde{X}^{\bar{U}}_{j} \tilde{X}^{\bar{S}}_{j}) \tilde{X}^{\bar{U}}_{a}) \tilde{V}_{\bar{R}\bar{S}}) \tilde{X}^{\bar{P}}_{a} \tilde{X}^{\bar{P}}_{i}) WXX^{\bar{P}\bar{R}} \quad (56)$$

$$E_{PH6} = \sum_{UV} (\sum_{em} (\sum_{Q} (\sum_{a} Q^{Q}_{am} \tilde{X}^{U}_{a}) (\sum_{j} \tilde{X}^{Q}_{j} \tilde{X}^{U}_{j}) \tilde{X}^{Q}_{e}) (\sum_{R} (\sum_{i} \bar{P}^{R}_{im} \tilde{X}^{V}_{i}) (\sum_{b} \tilde{\tilde{X}}^{R}_{b} \tilde{X}^{V}_{b}) \tilde{\tilde{X}}^{R}_{e})) T^{[1]}_{UV} \quad (57)$$

$$+ \sum_{\bar{U}\bar{V}} (\sum_{\bar{e}\bar{m}} (\sum_{\bar{Q}} (\sum_{\bar{a}} Q^{\bar{Q}}_{\bar{a}\bar{m}} \tilde{X}^{\bar{U}}_{a}) (\sum_{\bar{j}} \tilde{X}^{\bar{Q}}_{j} \tilde{X}^{\bar{U}}_{j}) \tilde{X}^{\bar{Q}}_{e}) (\sum_{\bar{R}} (\sum_{\bar{i}} \bar{P}^{\bar{R}}_{\bar{i}\bar{m}} \tilde{X}^{\bar{V}}_{i}) (\sum_{\bar{b}} \tilde{\tilde{X}}^{\bar{R}}_{b} \tilde{X}^{\bar{V}}_{b}) \tilde{\tilde{X}}^{\bar{R}}_{e})) T^{[1]}_{\bar{U}\bar{V}} \quad (58)$$

# Molecular Dynamics

To get the proper water solvation shell of 2H-2-azabicyclo[1.1.1]pentane, quantum mechanics/molecular mechanics (QM/MM) simulation was performed. The force field of 2-azabicyclo[1.1.1] pentane was generated by CgenFF tool.[1] The solute was first optimized at the B3LYP/def2-TZVP level with dispersion correction and was put in a sphere non-periodic water box of TIP3P waters with a minimum distance of 15 Angstrom between the box boundary and the solute. CHARMM with the CHARMM 36 force field[2] was used for 5000 steps of energy minimization to remove bad contacts and clashes. Semi-empirical QM/MM setup scheme[3,4]was adopted as the unavailability of accurate classical potentials for 2-azabicyclo[1.1.1]pentane. The semi-empirical QM potential, third-order Density Functional Tight Binding with 30b parameter set (DFTB3/3ob),[5] was used for the 2-azabicyclo[1.1.1]pentane. The rest of the system was modeled by the TIP3P water model. Simulations were integrated at 1.5 fs time steps. The SHAKE algorithm was applied to constrain the solvent molecules as rigid bodies. The nonbonding interaction cut-off was set at 12 Angstrom. 5000 steps of minimization, 30 ps of heating, 30 ps of equilibration, and finally a 300 ps production dynamic was performed using the hybrid DFTB3/3ob:CHARMM potential.[5] Then the last well-equilibrated

configuration was used to pick the water solvation shell. The closest 11 water molecules were selected and indexed by distance to 2-azabicyclo[1.1.1] pentane.

# References


(1) Vanommeslaeghe, K.; Hatcher, E.; Acharya, C.; Kundu, S.; Zhong, S.; Shim, J.; Darian, E.; Guvench, O.; Lopes, P.; Vorobyov, I.; Mackerell, J., A.D. CHARMM general force field: A force field for drug-like molecules compatible with the CHARMM all-atom additive biological force fields. *Journal of Computational Chemistry* **2009**, NA–NA.

(2) Best, R. B.; Zhu, X.; Shim, J.; Lopes, P. E. M.; Mittal, J.; Feig, M.; MacKerell, A. D. Optimization of the Additive CHARMM All-Atom Protein Force Field Targeting Improved Sampling of the Backbone $\phi$, $\psi$ and Side-Chain $\chi_1$ and $\chi_2$ Dihedral Angles. *Journal of Chemical Theory and Computation* **2012**, *8*, 3257–3273.

(3) Cui, Q.; Elstner, M.; Kaxiras, E.; Frauenheim, T.; Karplus, M. A QM/MM Implementation of the Self-Consistent Charge Density Functional Tight Binding (SCC-DFTB) Method. *The Journal of Physical Chemistry B* **2000**, *105*, 569–585.

(4) Gaus, M.; Cui, Q.; Elstner, M. DFTB3: Extension of the Self-Consistent-Charge Density-Functional Tight-Binding Method (SCC-DFTB). *Journal of Chemical Theory and Computation* **2011**, *7*, 931–948.

(5) Gaus, M.; Goez, A.; Elstner, M. Parametrization and Benchmark of DFTB3 for Organic Molecules. *Journal of Chemical Theory and Computation* **2012**, *9*, 338–354.
